# Supplementary material for: Carry Your Fault: A Fault Propagation Attack on Side-Channel Protected LWE-based KEM
Source: arXiv:2401.14098 source file (2024-01-25)
Supplement: Supplementary file 1 [file appendix.tex]

\section{Appendix} \label{sec:appendix}

\begin{algorithm}[!ht]
\caption{ Secure Arithmetic to Boolean conversion (A2B)~\cite{Coron2014_A2B} }
\label{algo:A2B1}

\Input{$\{A_i\}_{1\leq i \leq n}$ such that $\sum_{i=1}^{n} A_i = {x} \in \mathbb{R}_q $}
\Output{$\{y_i\}_{1\leq i \leq n}$ where each $ y_i \in \mathbb{R}_2^k$ and $\bigoplus_{i=1}^{n} y_i = x$}
\BlankLine
\If{$n=1$} {$y_1 \leftarrow A_1$\\ \algorithmicreturn{ $y_1$}} 
\Else{
$\{u_i\}_{1\leq i \leq \lfloor n/2\rfloor} \leftarrow \mathtt{A2B} (\{A_i\}_{1\leq i \leq \lfloor n/2\rfloor})$\\
$\{u_i\}_{1\leq i \leq n} \leftarrow \mathtt{RefreshXOR} (\{u_i\}_{1\leq i \leq \lfloor n/2\rfloor},n,k)$ [Algorithm \ref{algo:RefreshXOR}]\\
$\{v_i\}_{1\leq i \leq \lceil n/2\rceil} \leftarrow \mathtt{A2B} (\{A_i\}_{\lfloor n/2\rfloor + 1\leq i \leq n })$\\
$\{v_i\}_{1\leq i \leq n} \leftarrow \mathtt{RefreshXOR}(\{v_i\}_{1\leq i \leq \lfloor n/2\rfloor},n,k)$ [Algorithm \ref{algo:RefreshXOR}]\\
$\{y_i\}_{1\leq i \leq n} \leftarrow \mathtt{SecAdd}(\{u_i\}_{1\leq i \leq n},\{v_i\}_{1\leq i \leq n})$ [Algorithm \ref{algo:SecAdd1}]\\
\algorithmicreturn{ $\{y_i\}_{1\leq i \leq n}$}
}
\end{algorithm}

\begin{algorithm}[!ht]
\caption{ RefreshXOR~\cite{Coron2014_A2B}}
\label{algo:RefreshXOR}

\Input{$(\{x_i\}_{1\leq i \leq m}, n, k)$ where each $x_i \in \mathbb{R}_2^k$ and $\bigoplus_{i=1}^{m} x_i = x$}
\Output{$\{y_i\}_{1\leq i \leq n}$ with each $y_i \in \mathbb{R}_2^k$ such that $\bigoplus_{i=1}^{n} y_i = x$}
\BlankLine
\For{\texttt{i=1 to n}}
{
    $y_i\leftarrow x_i$\\
}
\For{\texttt{i=1 to n-1}}
{
   \For{\texttt{j=i+1 to n}}
    {
        $r\leftarrow \mathcal{U}(\mathbb{R}_2^k)$\\
        $y_i\leftarrow y_i\xor r$\\
        $y_j\leftarrow y_j\xor r$\\
    }
}
\algorithmicreturn{ $\{y_i\}_{1\leq i \leq n}$}

\end{algorithm}

\begin{algorithm}[!ht]
\caption{ SecAdd~\cite{Coron2014_A2B} }
\label{algo:SecAdd1}

\Input{$\{x_i\}_{1\leq i \leq n}$, $\{y_i\}_{1\leq i \leq n}$ with each $x_i,y_i \in \mathbb{R}_2^k$ such that $\bigoplus_{i=1}^{m} x_i = x$ and $\bigoplus_{i=1}^{m} y_i = y$}
\Output{$\{z_i\}_{1\leq i \leq n}$ where each $z_i \in \mathbb{R}_2^k$ and $\bigoplus_{i=1}^{m} z_i = x+y \mod{2^k}$}
\BlankLine
$\{c_i^{(0)}\}_{1\leq i \leq n}\leftarrow 0$\\
\For{\texttt{j=0 to k-2 }}
{
    $\{xy_i^{(j)}\}_{1\leq i \leq n} \leftarrow \mathtt{SecAnd}(\{x_i^{(j)}\}_{1\leq i \leq n},\{y_i^{(j)}\}_{1\leq i \leq n})$ [Algorithm \ref{algo:SecAnd}]\\
    $\{xc_i^{(j)}\}_{1\leq i \leq n} \leftarrow \mathtt{SecAnd}(\{x_i^{(j)}\}_{1\leq i \leq n},\{c_i^{(j)}\}_{1\leq i \leq n})$ [Algorithm \ref{algo:SecAnd}]\\
    $\{yc_i^{(j)}\}_{1\leq i \leq n} \leftarrow \mathtt{SecAnd}(\{y_i^{(j)}\}_{1\leq i \leq n},\{c_i^{(j)}\}_{1\leq i \leq n})$ [Algorithm \ref{algo:SecAnd}]\\
    $\{c_i^{(j+1)}\}_{1\leq i \leq n} \leftarrow \{(xy_i^{(j)})\}_{1\leq i \leq n}\xor \{(xc_i^{(j)})\}_{1\leq i \leq n}\xor \{(yc_i^{(j)})\}_{1\leq i \leq n}$\\
}
$\{z_i\}_{1\leq i \leq n} = \{x_i\}_{1\leq i \leq n} \xor \{y_i\}_{1\leq i \leq n} \xor \{c_i\}_{1\leq i \leq n}$ \\
\algorithmicreturn{ $\{z_i\}_{1\leq i \leq n}$}
\end{algorithm}

\begin{algorithm}[!ht]
\caption{ SecAnd~\cite{Coron2014_A2B} }
\label{algo:SecAnd}

\Input{$\{x_i\}_{1\leq i \leq n}$, $\{y_i\}_{1\leq i \leq n}$ with each $x_i,y_i \in \mathbb{R}_2^k$ such that $\bigoplus_{i=1}^{m} x_i = x$ and $\bigoplus_{i=1}^{m} y_i = y$}
\Output{$\{z_i\}_{1\leq i \leq n}$ where each $z_i \in \mathbb{R}_2^k$ and $\bigoplus_{i=1}^{m} z_i = x \wedge y $}
\BlankLine
\For{\texttt{i=1 to n}}
{
    $z_i\leftarrow x_i\wedge y_i$\\
}
\For{\texttt{i=1 to n-1}}
{
   \For{\texttt{j=i+1 to n}}
    {
        $r_{i,j}\leftarrow \mathcal{U}(\mathbb{R}_2^k)$\\
        $r_{j,i}\leftarrow (x_i\wedge y_j)\xor r_{i,j}$\\
        $r_{j,i}\leftarrow (x_j\wedge y_i)\xor r_{j,i}$\\
        $z_i\leftarrow z_i\xor r_{i,j}$\\
        $z_j\leftarrow z_j\xor r_{j,i}$\\
    }
}
\algorithmicreturn{ $\{z_i\}_{1\leq i \leq n}$}
\end{algorithm}
